# Supplementary material for: Mitigating Low-volume DoS Attacks with Data-driven Resource Accounting
Source: arXiv:2205.00056 source file (2022-04-29)
Supplement: Supplementary file 1 [file appendix.tex]

% \newpage
\appendix
\section{Configuration for evaluation}
\label{s:config}
% \XXX{Appendix is a candidate to move to supplementary material.}
\autoref{t:config} enumerates our default configuration
for evaluation.

\begin{table}[t]
  \vspace{0.7em}
  \centering
  \footnotesize
  \input{fig/config}
  \caption{Default configuration used for our evaluation.}
  \label{t:config}
%  \vspace{-5px}
\end{table}
%
%% \section{Adaptive Monitoring}
%% \begin{figure}[t]
%%   \centering
%%   \includegraphics[width=1.0\columnwidth]{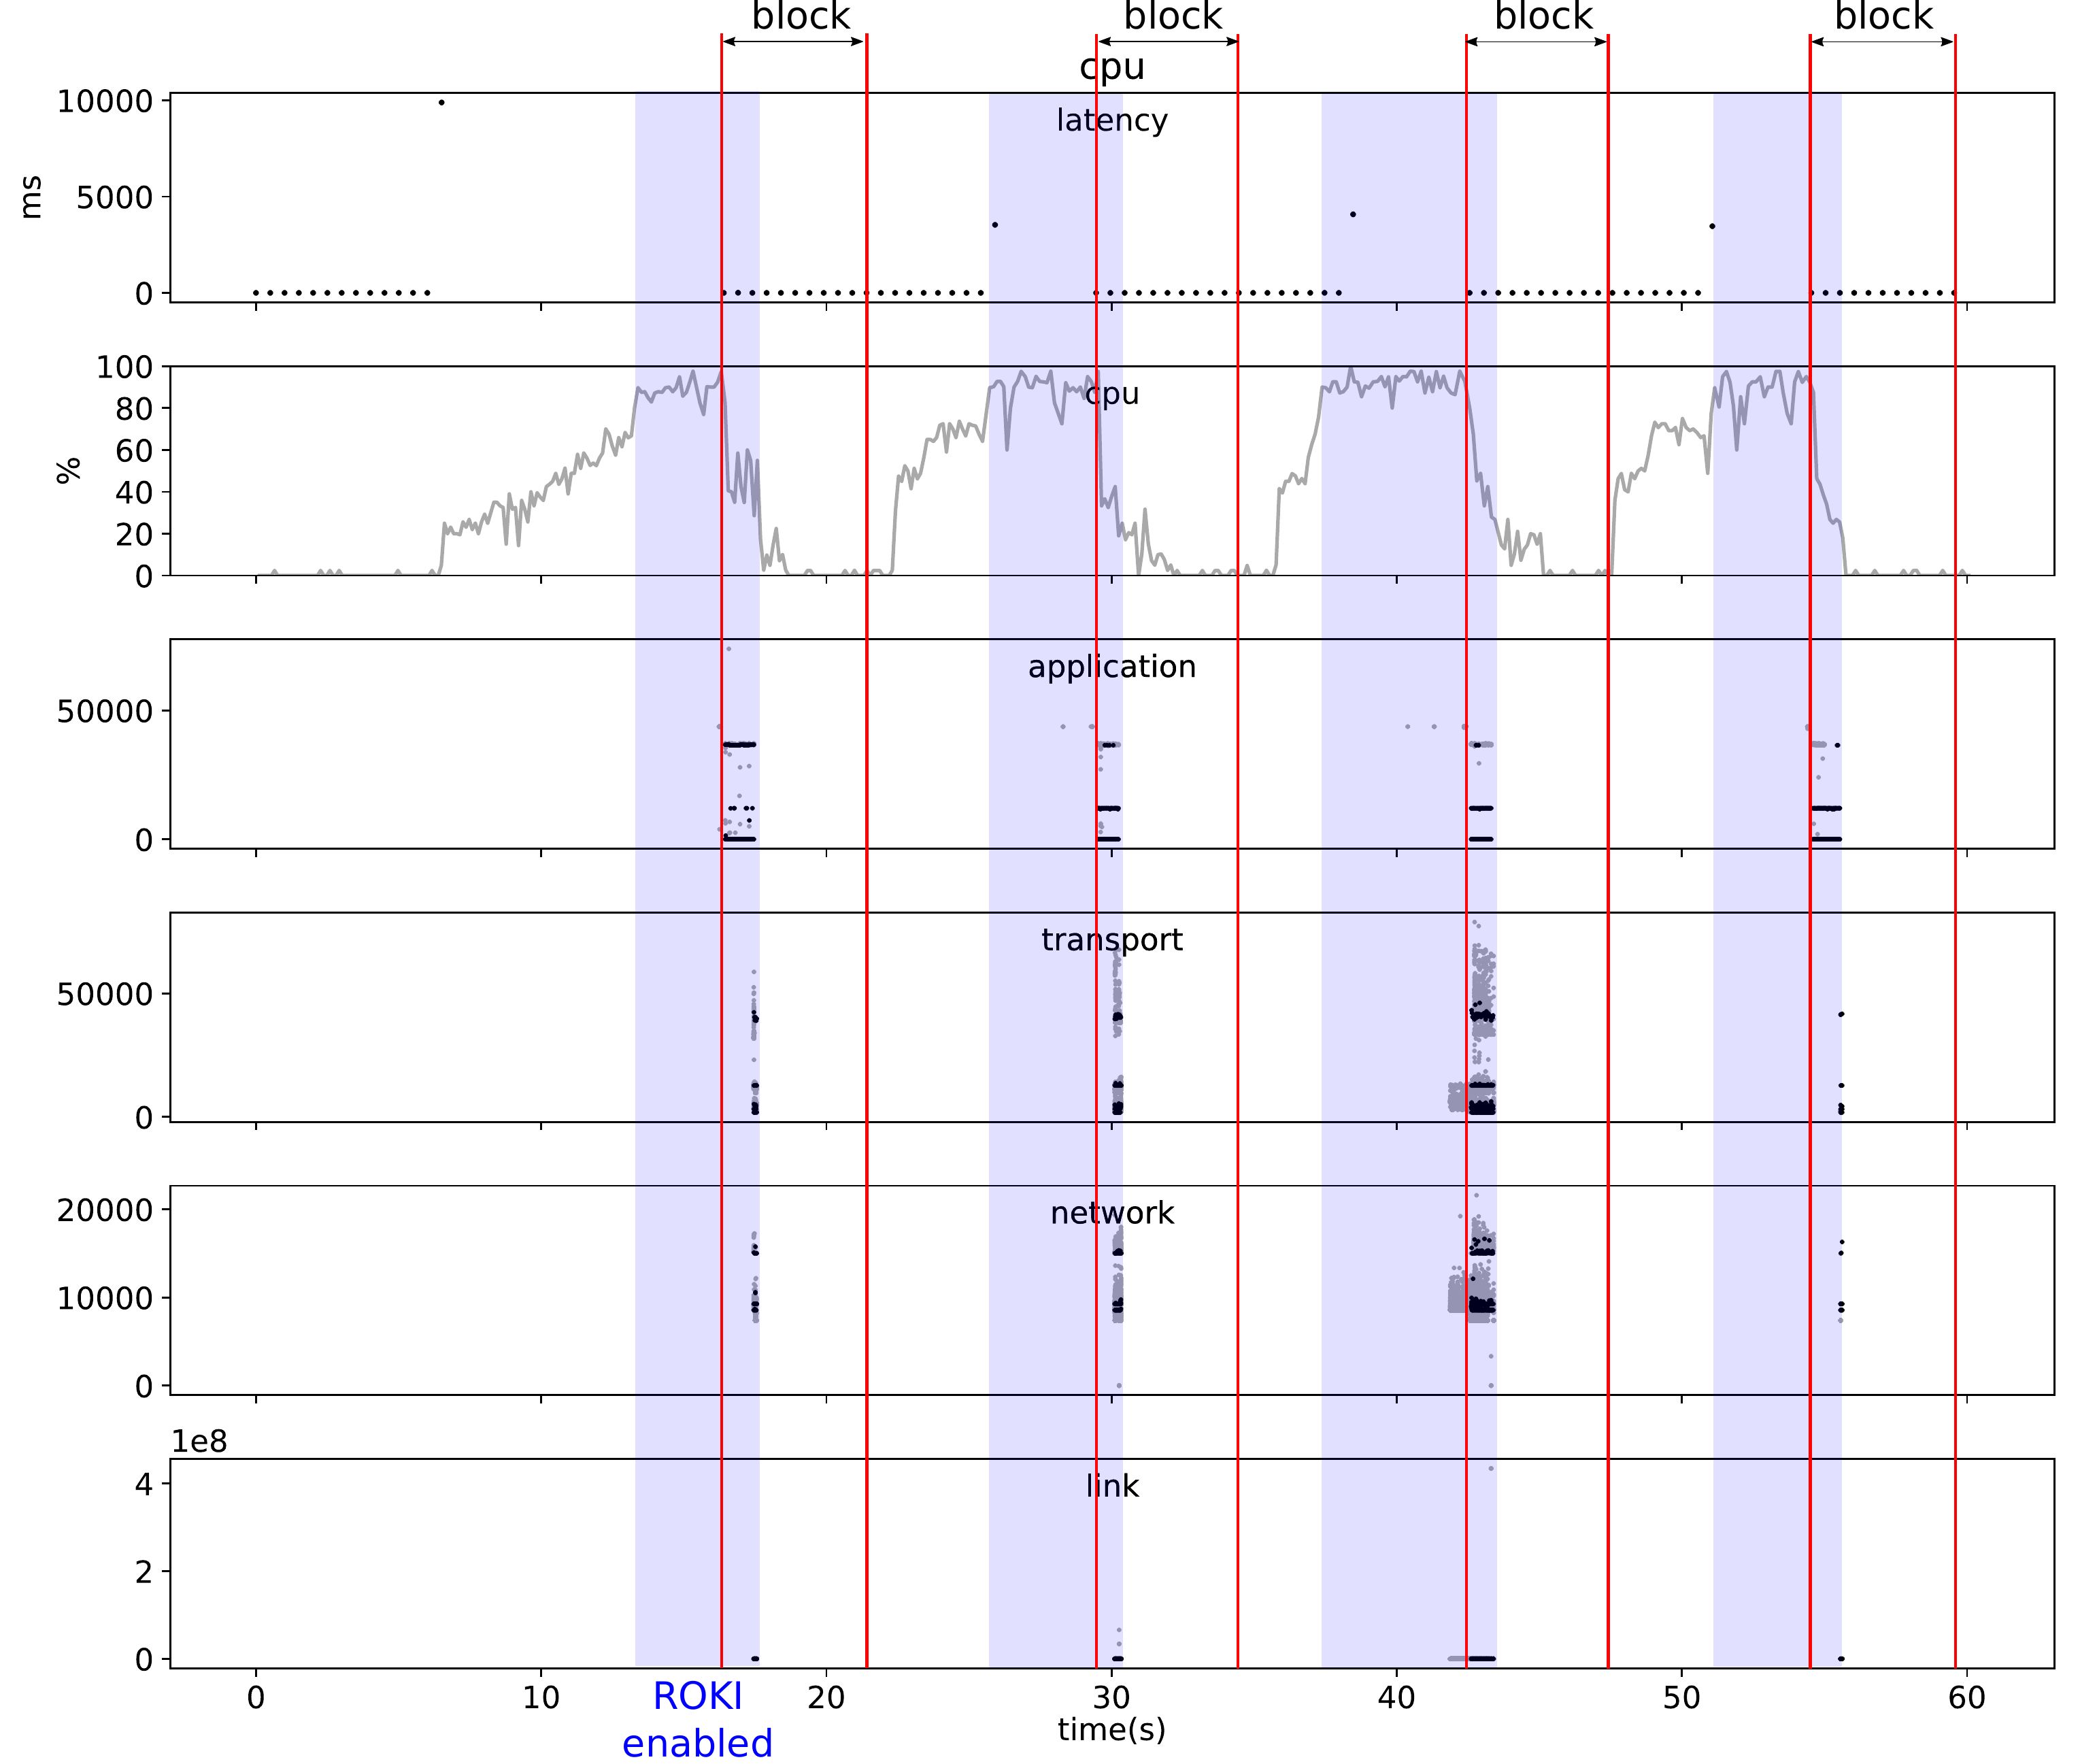}
%%   \caption{SSL/TLS renegotiation DoS attack under \sys with adaptive monitoring.
%%     The blue shade represents when \sys is active.
%%     When the attack used more than 75\% of the CPU resource,
%%     \sys was activated to avoid CPU exhaustion. When the CPU usage
%%     went below 35\%, \sys was deactivated to save
%%     resources. This feature helps lighten the overhead incurred
%%     by \sys.}
%%   \label{f:sslrenego-roki-cond-img}
%% \end{figure}
%% %
%% \autoref{f:sslrenego-roki-cond-img} shows how adaptive monitoring worked.
%% %
%% The blue shades in the figure represent when \sys was enabled and then disabled, and
%% the red lines display blocking time.
%% %
%% In this experiment,
%% \sys monitored the TLS/SSL renegotiation attack (\autoref{sss:sslrenego})
%% while using 75\% as the upper bound of CPU usage to activate \sys and
%% 35\% as the low bound of CPU usage to deactivate it.
%% %
%% The threshold to block clients were the same.
%% %
%% Once enabled,
%% \sys began profiling 2.5 second later due to initialization.
%% %
%% Adaptive monitoring conditionally activated \sys depending on
%% system resource usage. Therefore, when the system was not
%% overloaded, \sys did not consume any extra resources.
%% %

%\section{How request drops affect the latency improvement.}
\if 0
\section{Request drops versus Latency}
\label{s:availability}

\XXX{delete it or consider it as a supplement material}
%
% \XXX{service reliability for benign client?}
\sys aims to create a balance between
the number of request blocks and the overall QoS.
This is because it does not explicitly distinguish
low-volume DoS attacks from benign but expensive requests,
which is almost impossible.
Rather,
\sys temporarily blocks abnormal clients sending frequent expensive requests
to timely serve the requests from other normal clients.
Since this decision
allows \sys to block clients regardless of their intention,
it is worth to check the tradeoff between
the number of request blocks and the overall latency improvement.

% \sys's goal is not to accurately detect all low-volume DoS attacks. Rather, it
% focuses on mitigating the attack by blocking suspicious activities that abnormally
% consume much resources of system CPU, memory and connection pool. Regardless of
% client's intention, \sys would block her if her requests deplete resources more than
% the corresponding thresholds that the administrator set. Because of this approach,
% \sys could cause high false-positives or high false-negatives depending on the thresholds.
% However, we argue that this is trade-off that an administrator should pay.

% In this section, we would explore the relationship between false-positive and availability.

\PP{Methodology}
To evaluate the tradeoff between the number of request blocks and
the overall response time, we used three clients and a web server.
The server protected by \sys runs http-2.4.33
and its active cpu core is limited to two logical cores
in order to make the server handily saturated by three clients.
%whose configurations were mostly the same as those described in
%\autoref{sss:latency-throughput-methodology} except that only
%two logical cores of the server were enabled.
%
The three clients persistently requested a static page to
saturate the server's CPU. In addition, one of them monitored
response time from the server. While varying the threshold of
the number of the CPU instructions profiled at the application
layer, we measured the number of request drops incurred by \sys
and response time from the server for 60 seconds.
Note that two clients could be blocked but not the one that monitored
the response time.
%\SL{clearly two clients can be blocked, but the one monitoring response time would not}

\begin{figure}[t]
  \centering
  \includegraphics[width=\columnwidth]{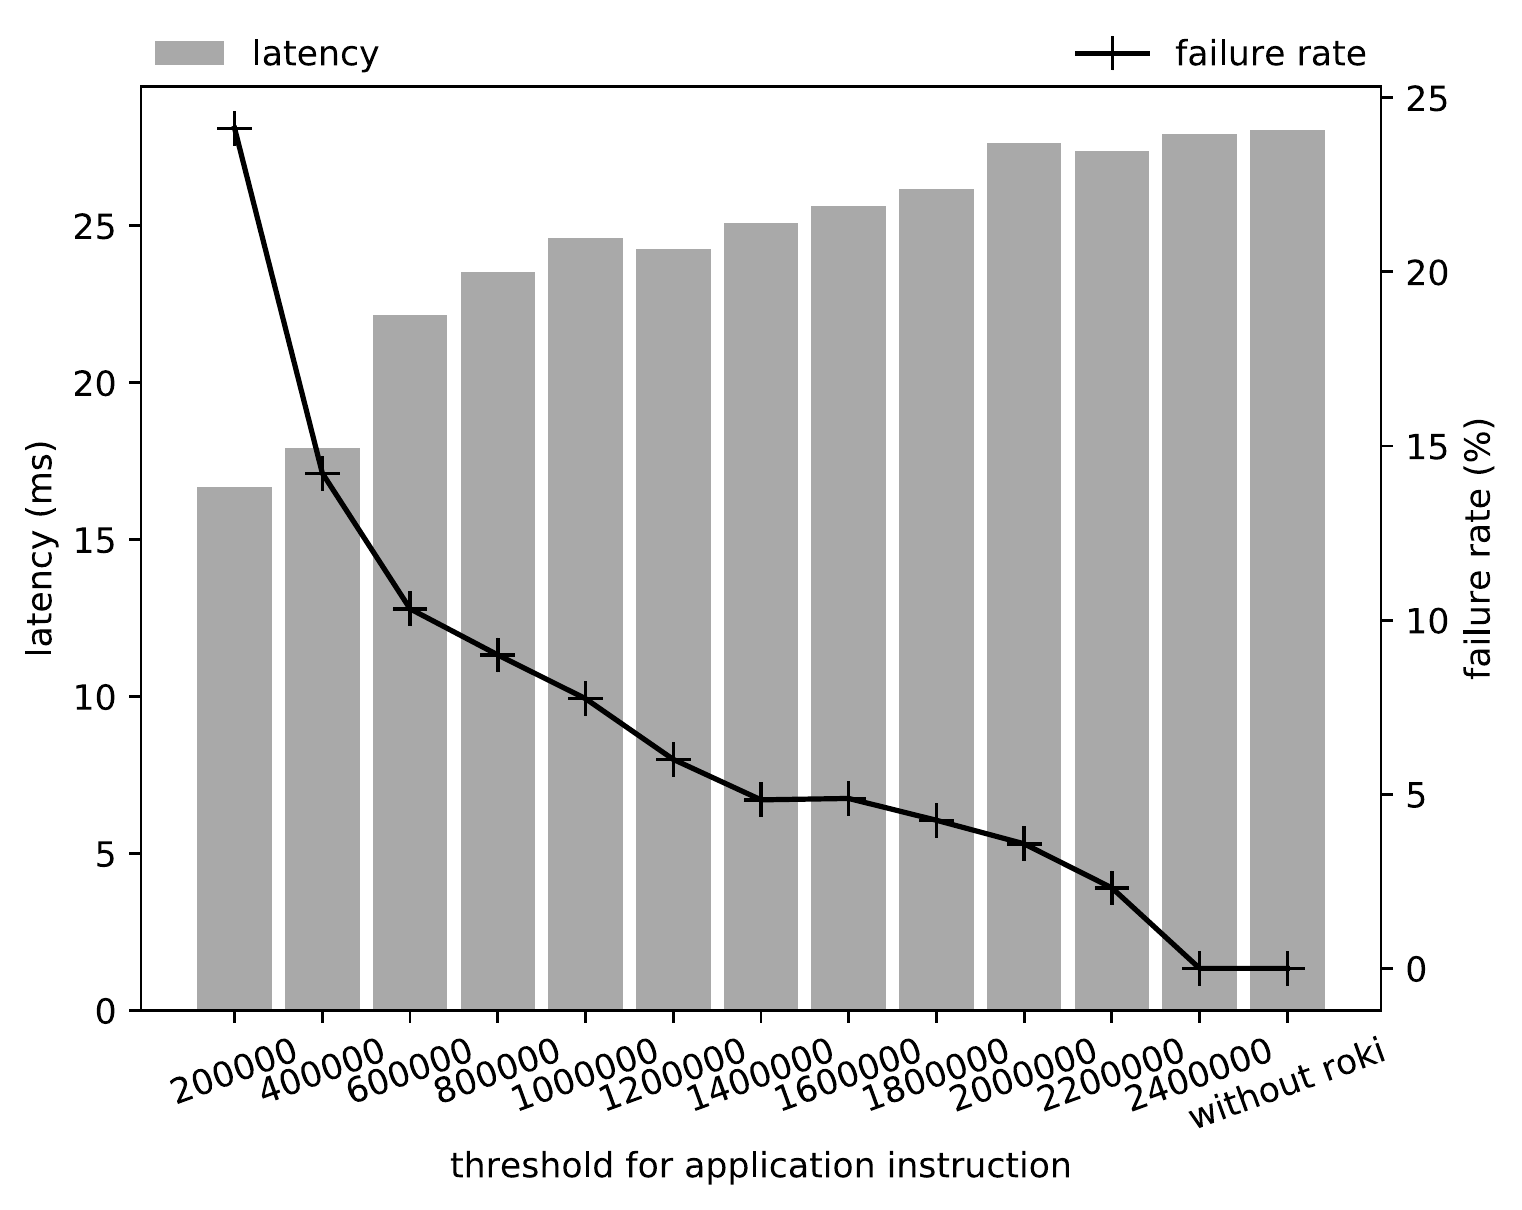}
  \caption{Average response time versus the number of blocks. They are inversely proportional.
    The more clients \sys blocks, the more time the server protected by \sys can serve in.}
  \label{f:fp-avail-img}
\end{figure}

\PP{Experimental results}
\autoref{f:fp-avail-img} shows the evaluation result.
The x-axis represents
the instruction threshold to block suspicious clients.
The left y-axis represents
average response time for requests of the monitor client during 60 seconds, and
the right y-axis represents
how many requests among all requests from the two other clients
were blocked by \sys during the experiment.
%\SL{put legend in the figure, not in the text.}
% The left and right y-axes represent response time of the server and the number of
% blocks incurred during the experiment respectively. The response time is represented
% as gray bars. And the number of blocks is drawn as a blue line graph.
%
Without \sys (the right-most bar),
the average of response time was 28 milliseconds.
In contrast,
with \sys and a threshold of 200,000 instructions,
the overall response time was improved to 17 milliseconds, but,
the request drop rate increased by 24.12\%.
With a threshold of 2,200,000 instructions,
the overall response time was 27 milliseconds while
request drop rate was 2.31\%.
%
% The right-most bar shows the processing time of the server without \sys.
% %
% With the 100,000 instruction threshold,
% the server consistently blocked two clients during the test and the total number
% of blocks was 41. A high number of blocks means that the server could have more time
% to serve other clients. This resulted in shorter processing time for the monitoring client.
% It could finish the test in just 143 second.
% On the other hand, with the instruction threshold of 1,700,000, the total number
% of blocks happened only three times but the total processing time for the monitor
% client to complete 1,000 requests became longer. It took 234 second.
%
We think that, at least for this experiment,
the optimal threshold lies between 1,400,000 and 1,600,000
to ensure both a small number of request drops and a short latency.
However,
the optimal threshold heavily depends on
system settings, workload, and, more importantly, the administrative policy:
serving all clients concurrently yet slowly or
serving some clients as early as possible and the other clients later.
%
% However,
% we could not argue that the threshold is the optimal value for every system.
% Because the optimal threshold could be different depending on the environment, applications
% and administrator's policy e.g., some administrators might prefer fairly serving
% all clients despite of longer latency or else the others might think serving more
% clients in the given time is better than serving all clients a poor service. Thus,
Thus,
we leave the decision of the optimal threshold to the discretion
of an administrator.

To wrap up our findings, as the server blocks more clients with a lower threshold,
the probability that benign clients are blocked might increase,
but the server timely serves more clients
since it can get more resources back by giving up some clients.
This approach is helpful for keeping the server available longer.
\fi
